# Supplementary material for: Beyond Expertise: Stable Individual Differences in Predictive Eye-Hand Coordination
Source: arXiv:2602.07816 source file (2026-04-07)
Supplement: Supplementary file 1 [file supplementary.pdf]

**Supplementary Figure S1. Individual trial examples of eye–hand coordination during the double via-point task.**

**Participant 1**

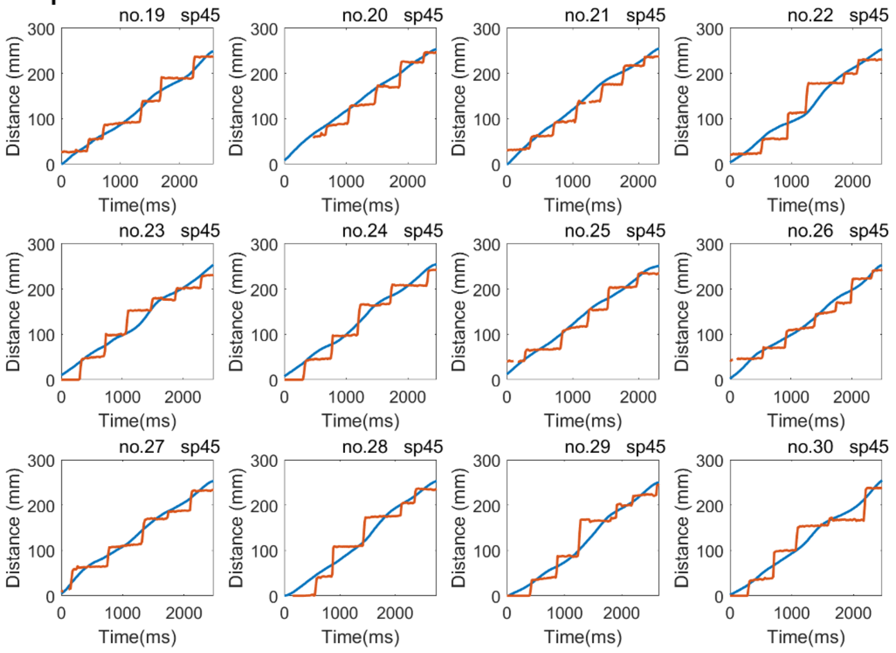


**Participant 2**

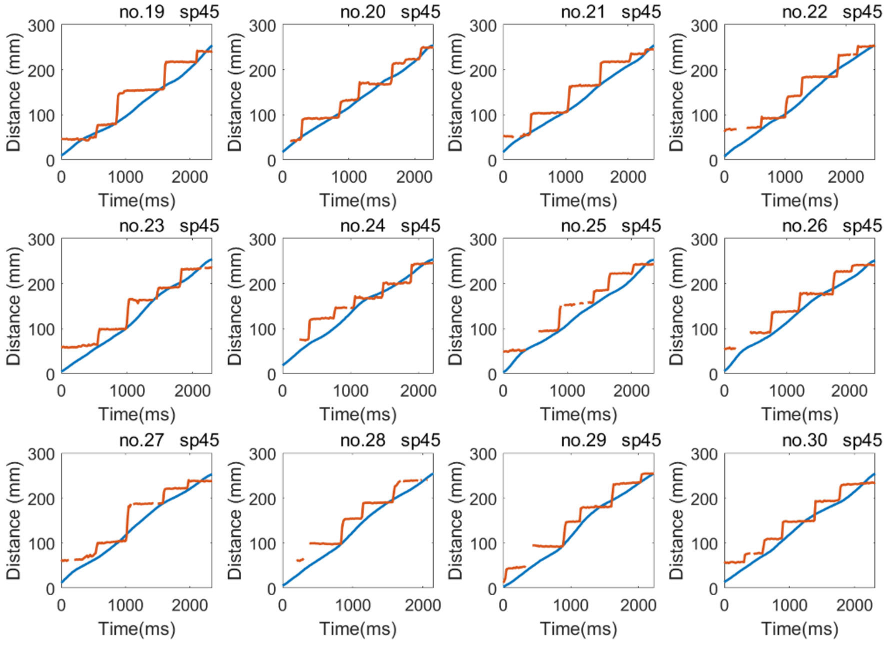

**Participant 3**

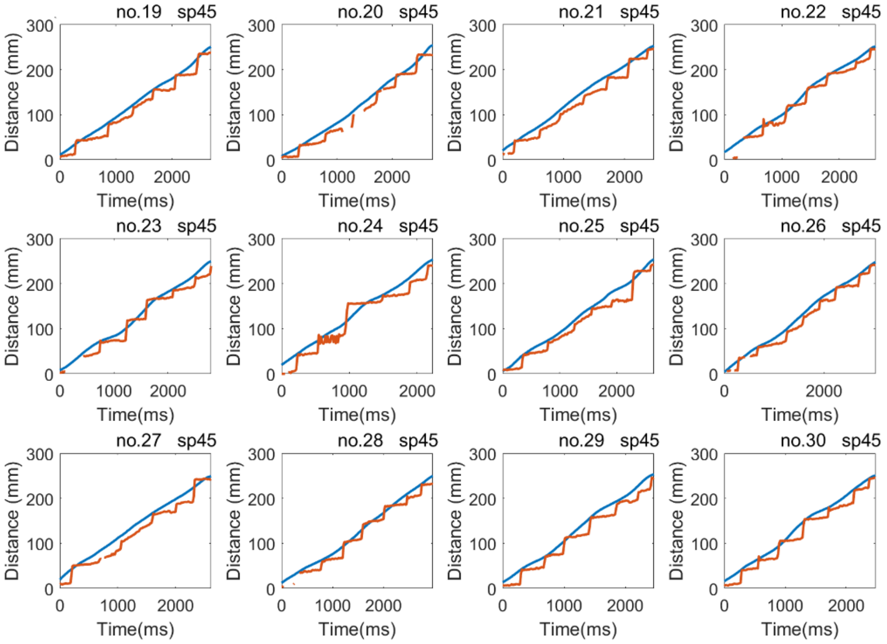


The panels display the temporal evolution of gaze (blue line) and pen (red line) positions for Participants 1, 2, and 3. Axes are consistent with Figure 2 (Time [ms] vs. Distance [mm]). The label above each plot identifies the specific trajectory type (e.g., no.19); identical numbers represent the same trajectory shape. All trials shown here correspond to the low speed condition (sp45). Note that while the gaze generally leads the pen via saccades in Participants 1 and 2, it sometimes lags behind the pen in Participant 3, highlighting the idiosyncratic nature of these predictive protocols.

**Supplementary Figure S2. Distribution of individual mean GP (mGP) and mean SD (mSD)**

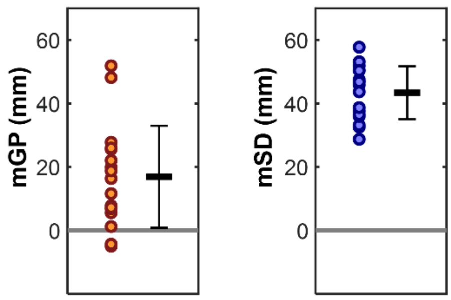


Each dot represents one participant. Horizontal bars indicate the group mean and standard deviation for each measure.
